# Supplementary material for: Beyond Linearity and Time-Homogeneity: Relational Hyper Event Models with Time-Varying Non-Linear Effects
Source: arXiv:2509.05289 source file (2025-11-29)
Supplement: Supplementary file 4 [file _SUPPLEMENTARY_FIGURE_RG_3.tex]

\begin{figure}
    \centering
    \begin{minipage}{0.45\linewidth}
        \centering
        \includegraphics[width=\linewidth]{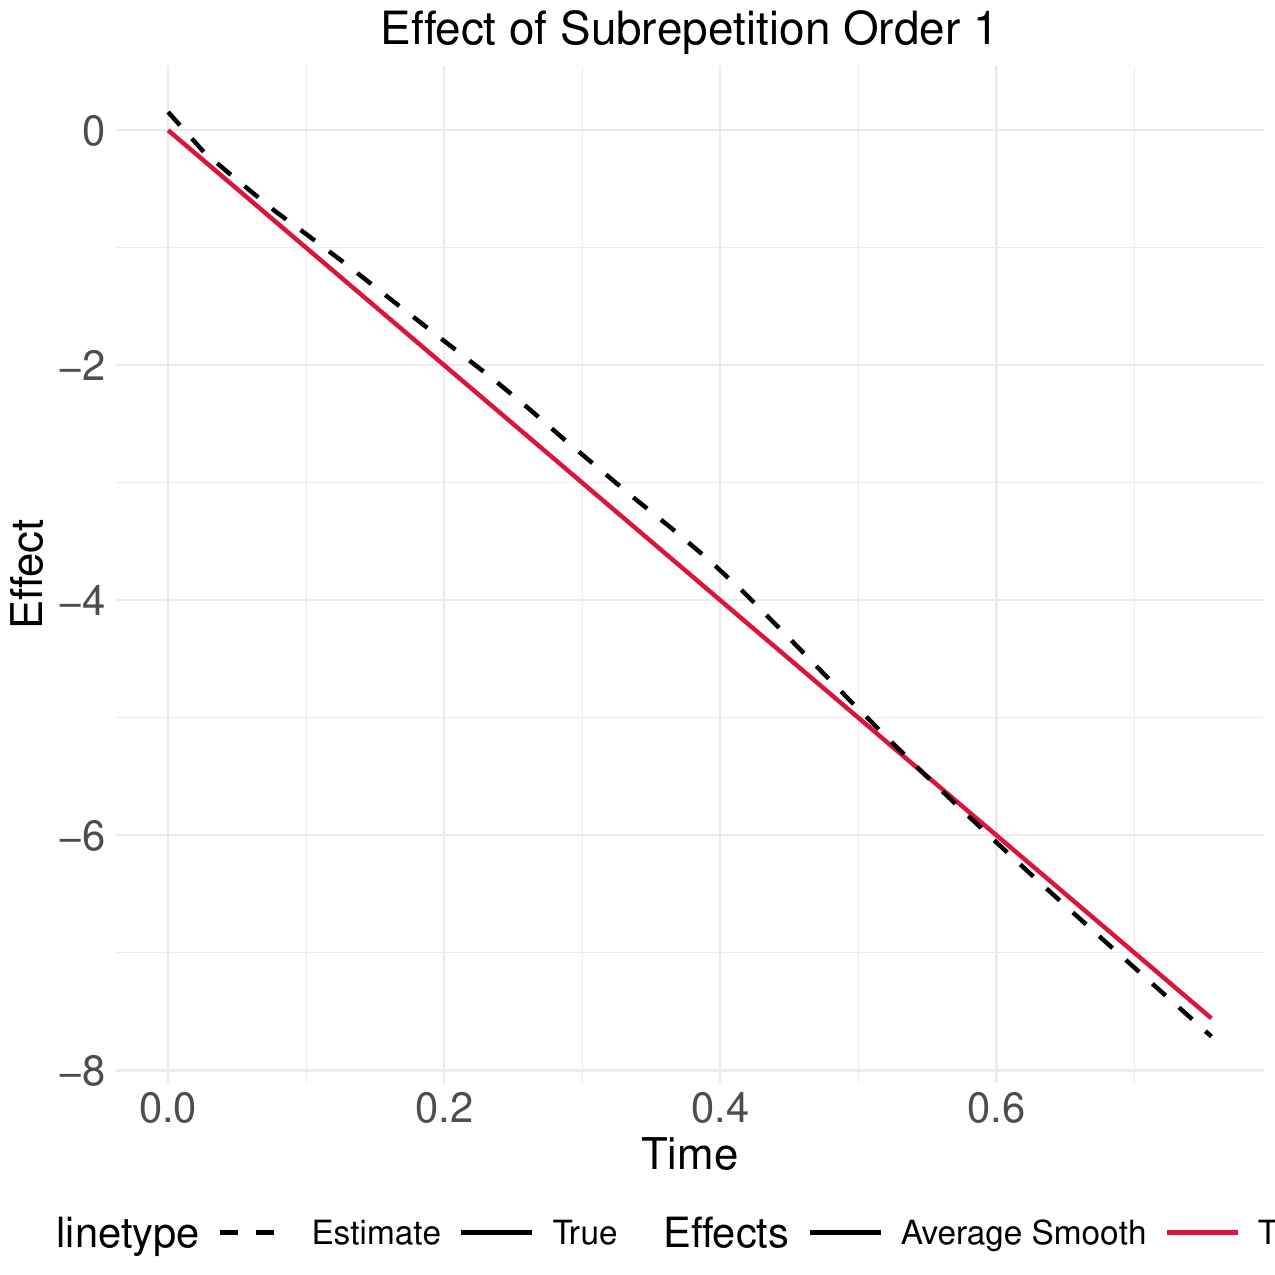}
    \end{minipage}
    \begin{minipage}{0.45\linewidth}
        \centering
        \includegraphics[width=\linewidth]{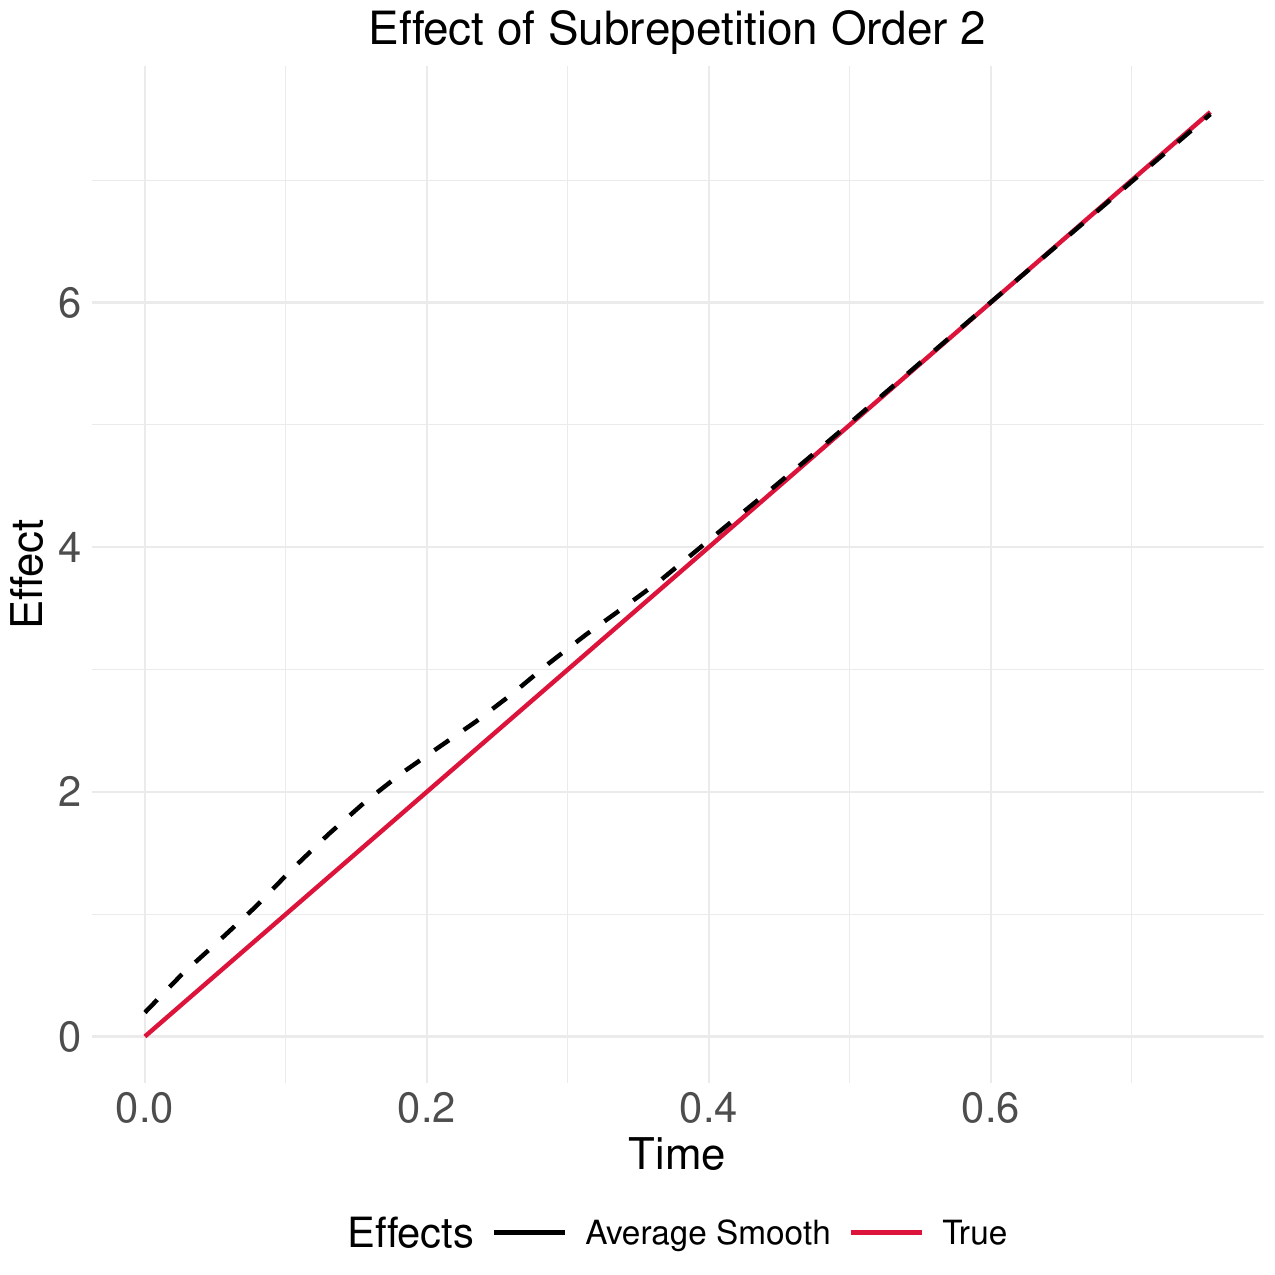}
    \end{minipage}
    \caption{\label{fig:simulation_study_tvnle_supplementary}%
    \textbf{Time-varying effects for sub-repetition covariates}. This figure shows the estimated effects for the order 1 and 2 sub-repetition covariates within the model that includes TVNLE. These covariates are transformed using the log-square root function, as in the previous section. Their effect remains purely time-varying.}
\end{figure}
